# Supplementary material for: Robust and bright polarization-entangled photon sources exploiting non-critical phase matching without periodic poling
Source: arXiv:2409.07673 ancillary file (2024-09-12)
Supplement: Supplementary file 1 [file NCPM_supplement_v6_LSA.pdf]

# Supplementary Information - Robust and bright polarization-entangled photon sources exploiting non-critical phase matching without periodic poling

Ilhwan Kim,[1,2] Yosep Kim,[3] Yong-Su Kim,[1,4] Kwang Jo Lee,[2,*] and Hyang-Tag Lim[1,4,†]

[1] *Center for Quantum Technology, Korea Institute of Science and Technology (KIST), Seoul, 02792, Korea*
[2] *Department of Applied Physics, Kyung Hee University, Yongin-si 17104, Korea*
[3] *Department of Physics, Korea University, Seoul 02841, Korea*
[4] *Division of Quantum Information, KIST School, Korea University of Science and Technology, Seoul 02792, Korea*

* kjlee88@khu.ac.kr
† hyangtag.lim@kist.re.kr

# I. SUPPLEMENTARY NOTE 1 - CALCULATION DETAILS

## A. Type-II NCPM in a KTP crystal

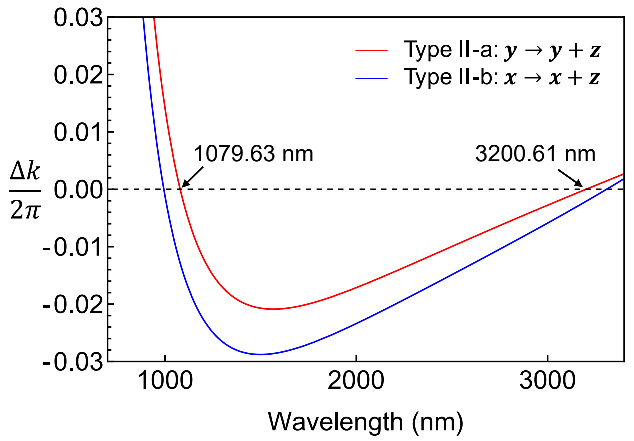


Supplementary Figure 1. **Phase mismatch in frequency-degenerate Type-II spontaneous parametric down-conversion (SPDC) in a bulk KTP as a function of the photon-pair wavelengths.** The two curves represent two kinds of Type-II interactions: Type-II-a and Type-II-b. The four points where the dashed line (corresponding to $\Delta k = 0$) intersects the two curves indicate the wavelengths that satisfy non-critical phase matching (NCPM). The interaction of photons is expressed as pump $\rightarrow$ signal + idler, where $x$, $y$ and $z$ represent the polarization direction of the photons with respect to the optical axes of the KTP crystals. The perfect NCPM condition is satisfied at a wavelengths of 1079.63 (991.89) nm and 3200.61 (3325.99) nm for the Type-II-a (Type-II-b) interaction.

We investigated characteristics of the Type-II non-critical phase matching (NCPM) in a bulk potassium titanyl phosphate (KTP) crystal in terms of the spectral position of generated photons, corresponding spectral bandwidth and spatial walk-offs. We considered frequency-degenerate case to achieve the high spectral purity of generated polarization-entangled two-photon states. The condition for Type-II frequency-degenerate NCPM is as follows:

$$\Delta k = k_p^{(\alpha)} - k_s^{(\alpha)} - k_i^{(\beta)} = 0, \tag{1}$$

where each $k$ corresponds to the wave number of the interacting photons and subscripts $p, s$, and $i$ refer to the pump, signal, and idler, respectively. Superscripts $\alpha$ and $\beta$ denote the polarization directions of photons corresponding to the one of the optical axes $(x, y, z)$ of the KTP crystal. In Eq. (1), wavelengths of the down-converted signal photon and idler photons are identical ($\lambda_s = \lambda_i$), whereas their polarization directions are orthogonal to each other, resulting in a difference between their $k$. In a bulk KTP crystal, $yyz$ (Type-II-a) and $xxz$ (Type-II-b) conditions are possible. The propagating directions of the interacting photons in Type-II-a and Type-II-b interactions are parallel to $x$-axis and $y$-axis of a KTP crystal, respectively. Supplementary Figure 1 shows the phase mismatches for the Type-II-a and Type-II-b NCPM conditions as a function of the wavelength of the down-converted photon $\lambda_s$. In order to calculate the NCPM condition in a KTP crystal, we used the Sellmeier equations from Ref. [1] for $y, z$ components and from Ref. [2] for $x$ component. The temperature of the KTP crystal is set to 30°C. The SPDC process occurs when NCPM condition $\Delta k = 0$ is satisfied and generates photon pairs at a wavelength of $\lambda_s$. We obtained two similar phase matched wavelength $\lambda_s$ from the two NCPM conditions, respectively.

When we choose an interaction type for SPDC process, we consider the magnitude of the effective nonlinear optical coefficient ($d_{\text{eff}}$), as the square of it is proportional to the photon generation rate ($\eta_{\text{SPDC}}$) in the SPDC process. $d_{\text{eff}}$ for the Type-II-a and Type-II-b interactions are $d_{24} = 3.75$ and $d_{15} = 2.02$, respectively. It means that the SPDC process with Type-II-a NCPM in a bulk KTP crystal generates 3.44 times more photon pairs than in the case of the Type-II-b NCPM. Thus, we exploited the Type-II-a NCPM technique to generate a polarization-entangled photon pairs via the SPDC process in a bulk KTP crystal.

## B. Spectral bandwidth of down-converted photons

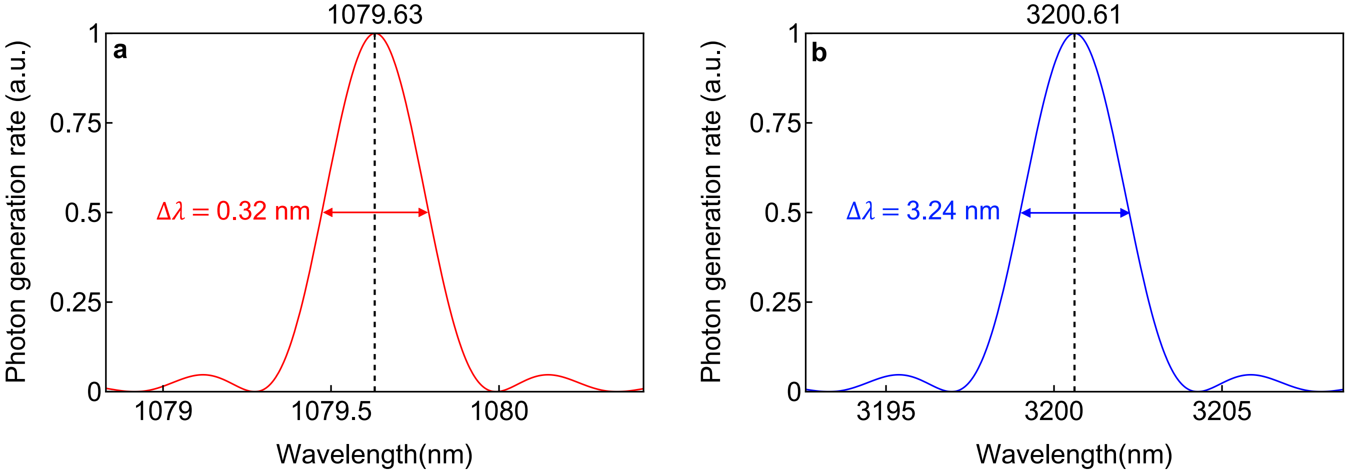


Supplementary Figure 2. **Spectra of the normalized photon generation rate.** We consider the SPDC process via Type-II-a NCPM in a 20-mm-long bulk KTP crystal. The generated photons are at the center wavelength of perfectly phase matched wavelengths **a,** 1079.63 nm and **b,** 3200.61 nm, as shown in Supplementary Fig. 1. The obtained full-width-half-maximums (FWHMs) are 0.32 nm and 3.24 nm for **a** and **b**, respectively.

We can expect the spectral bandwidth of photons generated via SPDC by using the function of $\eta_{\text{SPDC}}$ corresponding to the phase mismatch $\Delta k$. $\eta_{\text{SPDC}}$ for the frequency-degenerate Type-II-a NCPM is expressed as follows:

$$\eta_{\text{SPDC}} \propto d_{24}^2 \text{sinc}^2(\frac{\Delta k_{24} L}{2}), \tag{2}$$

with

$$\Delta k_{24} = \frac{2\pi}{\lambda_s}\left[2n_y(\frac{\lambda_s}{2}) - n_y(\lambda_s) - n_z(\lambda_s)\right], \tag{3}$$

where $L$ refers to the length of a crystal and $\Delta k_{24}$ means phase mismatch in a Type-II-a NCPM condition. The relation $\lambda_p = 2\lambda_s$ is given by the energy conservation of the SPDC process. We plotted the spectra of the normalized $\eta_{\text{SPDC}}$ as a function of $\lambda_s$ at a wavelengths of 1079.63 nm and 3200.61 nm as shown in Supplementary Fig. 2**a** and **b**, respectively. The down-converted photons at a center wavelength of 1079.63 nm show 10 times narrower full-width-half-maximum (FWHM) than those at 3200.61 nm. Note that the wavelength of 1079.63 nm lies within the optical communication T-band, which is employed in free space communication and light detection and ranging (LIDAR) system due to its high performance in atmospheric propagation and high photon detection efficiency [3–5]. In this work, we generate the photon pairs at 1079.63 nm nm via the SPDC process with Type-II NCPM for preparing polarization-entangled photon pairs.

## C. Angular tolerance and spatial walk-off

We estimated the robustness of $\eta_{\text{SPDC}}$ against to misalignment of the pump beam in a bulk KTP crystal for Type-II NCPM and compared results with the QPM case in a PPKTP crystal. Supplementary Figure 3**a** shows normalized $\eta_{\text{SPDC}}$ as a function of $\phi$ and $\theta$ corresponding to polar and azimuthal angles between the propagating direction of the pump beam and the $x$-axis of a KTP crystal, respectively. $\eta_{\text{SPDC}}$ shows FWHMs of 1.78° and 4.66° for the misalignment of the pump beam in $\theta$ and $\phi$ direction, respectively. When a photon propagates within a birefringent crystal along a direction that is not parallel to the axis of the crystal, a separation between the wave vector and the Poynting vector occurs, so called spatial walk-off. For given photon at a center wavelength of $\lambda$, the spatial walk-off $\rho$ in a KTP crystal can be expressed by

$$\tan\rho_{\lambda,m} = n_{s,m}^2(\lambda)\left[\left(\frac{s_x}{n_{s,m}^{-2}(\lambda) - n_x^{-2}(\lambda)}\right)^2 + \left(\frac{s_y}{n_{s,m}^{-2}(\lambda) - n_y^{-2}(\lambda)}\right)^2 + \left(\frac{s_z}{n_{s,m}^{-2}(\lambda) - n_z^{-2}(\lambda)}\right)^2\right]^{-\frac{1}{2}}, \tag{4}$$

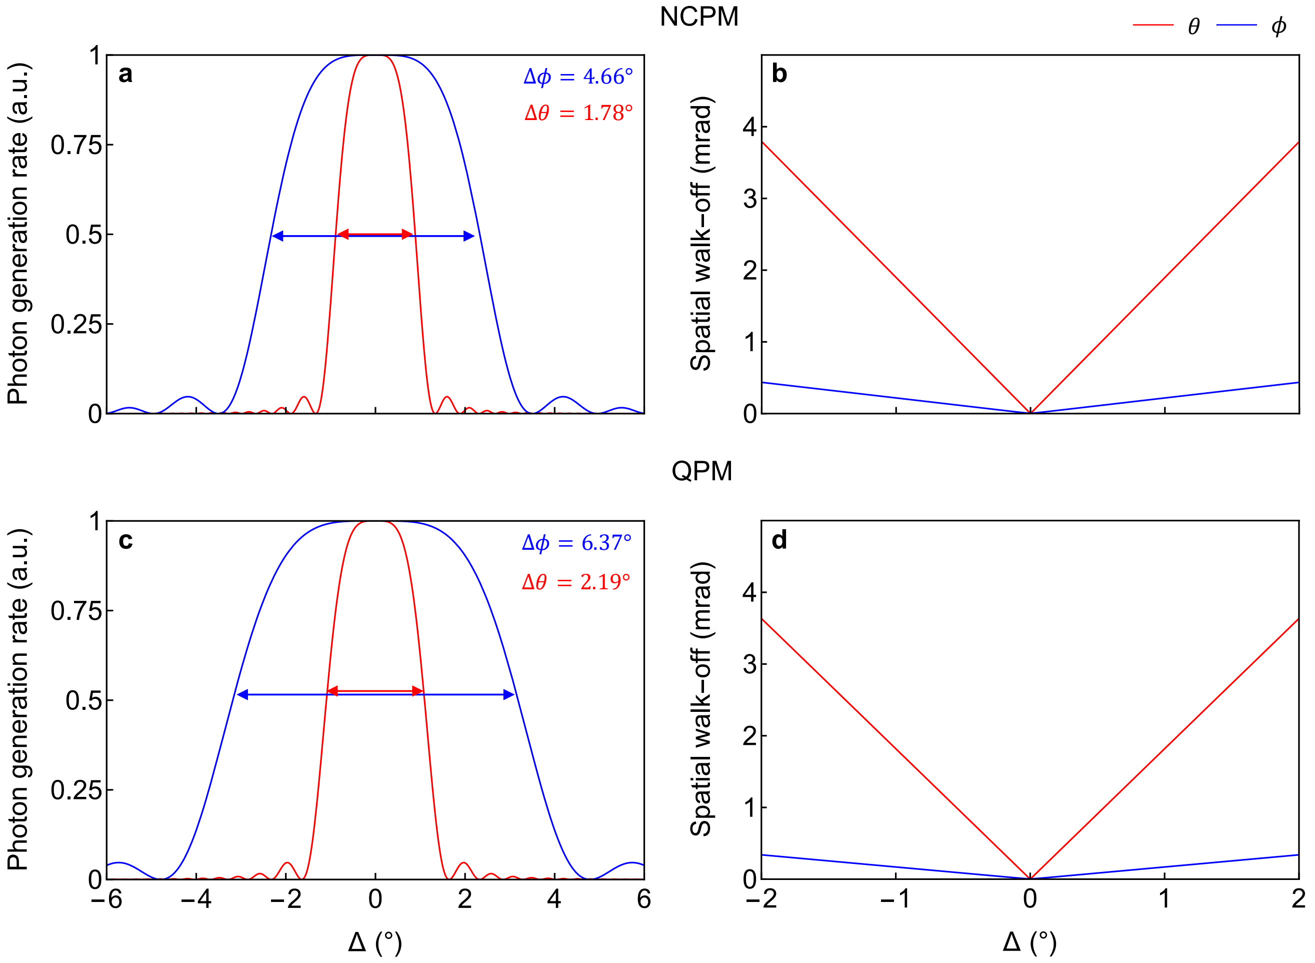


Supplementary Figure 3. **Robustness of the SPDC process against misalignment of the pump beam in a KTP crystal and a PPKTP crystal. a,** The angular tolerances of the normalized SPDC conversion efficiency and **b,** the spatial walk-offs among interacting photons for the Type-II NCPM in a 20-mm-long bulk KTP crystal. $\Delta$ refers to the misalignment of the pump beam in the directions of $\theta$ and $\phi$. The FWHMs of the angular tolerance are 1.78° and 4.66° for misalignment in the $\theta$ and $\phi$ directions, respectively. The spatial walk-offs are 4.0 mrad and 0.43 mrad for misalignment of the pump beam by 2.0° (35 mrad) in the $\theta$ and $\phi$ directions, respectively. The calculated **c,** angular tolerances and **d,** spatial walk-offs for the Type-II QPM interaction in a 20-mm-long PPKTP crystal designed to generate photon pairs at 1560 nm. The FWHM of angular tolerance and the spatial walk-off at the $\Delta$ = 35 mrad are 2.19° (6.37°) and 3.6 (0.34) mrad in the $\theta$ ($\phi$) direction, respectively.

where $\boldsymbol{s}(s_x, s_y, s_z)$ refers to the propagating direction of the photon and $n_{\boldsymbol{s},m}$ is the refractive index (RI) in the direction $\boldsymbol{s}$ [6]. $m$ can be $l$ or $h$, denoting low or high RI for given $\boldsymbol{s}$ and $\lambda$. For the Type-II PM interaction, the spatial walk-off ($w$) is defined as the largest angle between Poynting vectors of the interacting photons. It can be expressed by

$$\cos w = \cos \rho_{\lambda_p,h} \cos \rho_{\lambda_s,l}. \tag{5}$$

We plotted $w$ as a function of $\phi$ and $\theta$ in Supplementary Fig. 3**b**. When misalignment of 2.0° (35 mrad) is introduced, the largest spatial walk-off angle between photons is 0.23° (4.0 mrad). Thus, spatial walk-off effect is negligible. Supplementary Figure 3**c** and **d** show $\eta_{\text{SPDC}}$ and $w$ as a function of $\phi$ and $\theta$ for Type-II QPM interaction in a PPKTP crystal, respectively. We assumed the poling period of the KTP crystal as 46.165 μm so that the center wavelength of the generated photon pair is 1560 nm at 30°C. We estimated the FWHMs of $\eta_{\text{SPDC}}$ as $\Delta\theta_{\text{PP}} =$ 2.19° and $\Delta\phi_{\text{PP}} =$ 6.37°, and the spatial walk off as 3.6 mrad and 0.34 mrad at a 35 mrad misalignment in the $\phi$ and $\theta$ directions, respectively. It shows that the Type-II NCPM has similar robustness properties with QPM.

### D. Joint spectral analysis

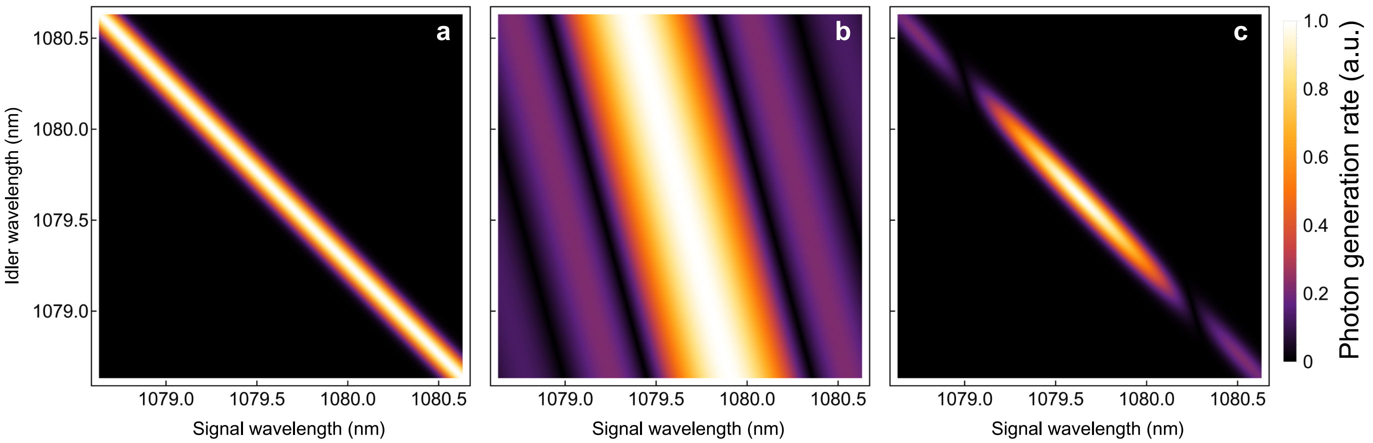


Supplementary Figure 4. **The joint spectral analysis of the photon pairs generated via SPDC process with Type-II NCPM in a bulk KTP crystal.** The theoretical **a,** pump envelop (PE) function, **b,** phase matching function and corresponding **c,** joint spectral amplitude (JSA). We considered pump beam with root mean square (RMS) width of 0.022 nm and a 20-mm-long bulk KTP crystal.

We performed a joint spectral analysis, including a theoretical simulation of the joint spectral amplitude (JSA) of the two-photon state generated using the Type-II NCPM technique and a calculation of the spectral purity of the photon pairs via Schmidt decomposition. The two-photon state generated via the SPDC process is expressed as follows:

$$|\Phi\rangle = \int_0^\infty \int_0^\infty d\lambda_s d\lambda_i f(\lambda_s, \lambda_i) \hat{a}_s^\dagger(\lambda_s) \hat{a}_i^\dagger(\lambda_i) |0\rangle|0\rangle, \tag{6}$$

where $\hat{a}_s^\dagger$ and $\hat{a}_i^\dagger$ are creation operator of signal and idler photons, respectively.

Correlation function $f(\lambda_s, \lambda_i)$ represents JSA, which is the product of the pump envelop (PE) function $\alpha(\lambda_s, \lambda_i)$ and the PM function $\phi(\lambda_s, \lambda_i)$. JSA can be expressed by

$$f(\lambda_s, \lambda_i) = \alpha(\lambda_s, \lambda_i)\phi(\lambda_s, \lambda_i). \tag{7}$$

We used the second harmonic (SH) beam generated from the PPLN crystal as a pump beam. Theoretically, the generated SH beam has a sinc-squared spectral shape with a root mean square (RMS) width of 0.022 nm. To simplify analytical condition, we assumed the PE function of the pump beam to be Gaussian with a RMS width of 0.022 nm and a center wavelength of 1079.63 nm, which corresponds to the perfectly phase matched wavelength. Then, the PE function is as follows:

$$\alpha(\omega_s, \omega_i) \propto \exp\left[-\frac{(\omega_s + \omega_i - \omega_p)^2}{2\sigma_p^2}\right], \tag{8}$$

where $\omega = \frac{2\pi c}{\lambda}$ and $\sigma_p$ indicates the RMS width of the the pump beam. In our work, the PM function is given by:

$$\phi(\lambda_s, \lambda_i) \propto \mathrm{sinc}\left(\frac{\Delta k_{24} L}{2}\right), \tag{9}$$

where $\Delta k_{24}$ is the phase mismatch for the Type-II NCPM condition, as given by Eq. (3) and $L$ refers to the crystal length. Here, we use $L$ = 20 mm, which corresponds to our experimental condition. Supplementary Figure 4**a-c** shows density plots of the PE function, PM function, and corresponding JSA as a function of $\lambda_s$ and $\lambda_i$, respectively.

Then, we calculated spectral purity of the generated photon pairs. The spectral purity of the two-photon state is obtained via Schmidt decomposition of the correlation function:

$$f(\lambda_s, \lambda_i) = \sum_j \sqrt{c_j} |\zeta_{s,j}\rangle |\zeta_{i,j}\rangle, \tag{10}$$

where $c_j$ represents Schmidt coefficient. $c_j$ is composed of non-negative real values, satisfying the normalization condition $\sum_j c_j = 1$. $|\zeta_{s,j}\rangle$ and $|\zeta_{i,j}\rangle$ denote Schmidt modes, corresponding to the orthonormal basis states. Then, we can calculate the spectral purity $P$ as given by:

$$P = \sum_j c_j^2. \tag{11}$$

From the obtained JSA as shown in Supplementary Fig. 4**c**, We calculated the spectral purity of the generated photon pairs to be 0.979.

## II. SUPPLEMENTARY NOTE 2 - EXPERIMENTAL DETAILS

### A. Second harmonic generation

To confirm that the SPDC process with Type-II NCPM in a bulk KTP crystal can produce frequency-degenerate photon pairs, we utilized the second harmonic generation (SHG), which is the reverse process of SPDC. In the SHG process, a $y$-polarized SH beam is obtained by pumping a bulk KTP crystal with $y$- and $z$-polarized pump

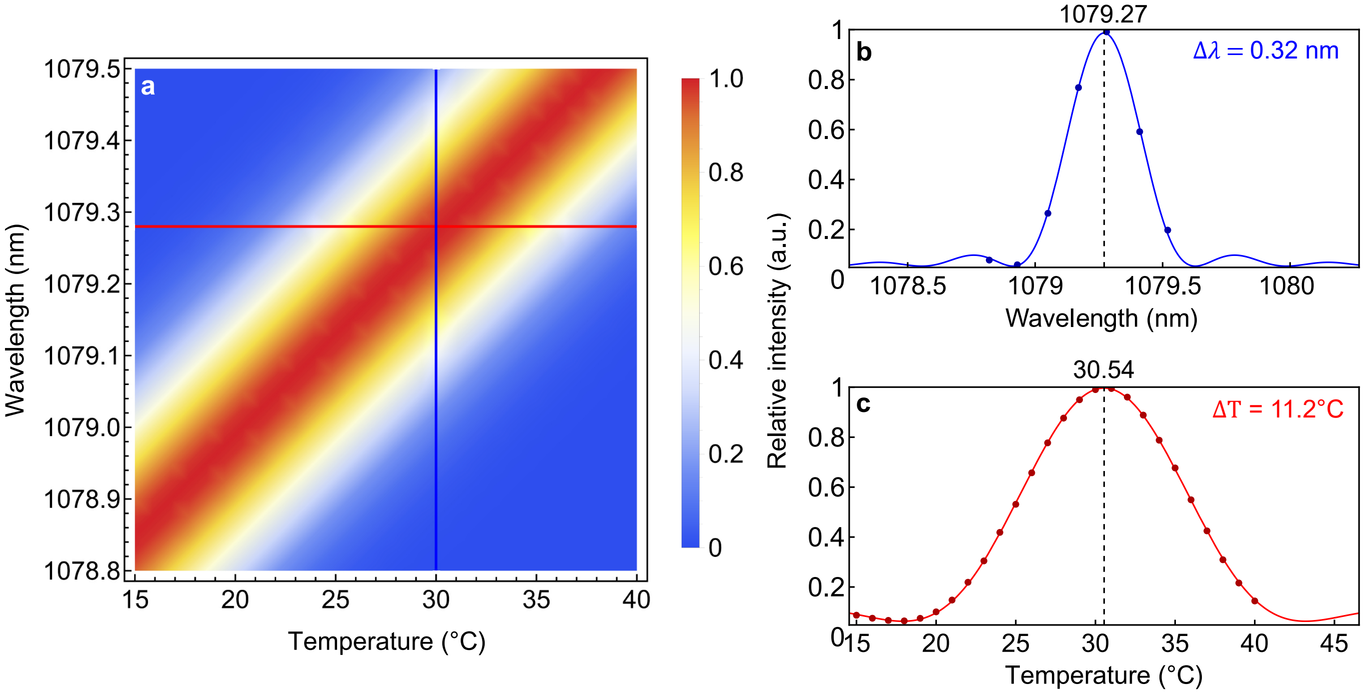


Supplementary Figure 5. **Experimental results of second harmonic generation (SHG) in a bulk KTP crystal. a,** A 2D density plot of the function fitted from the SHG conversion efficiency as a function of the pump laser wavelength and temperature of the KTP crystal. The SHG conversion efficiency is defined as the measured power of the SH beam divided by the power of the pump laser, which is 0.8 W. **b,** Measured SHG conversion efficiency (dots) and the corresponding fitting function (solid line) obtained as the laser wavelength varied while the crystal temperature was fixed at 30°C. The center wavelength of 1079.27 nm with an FWHM of 0.32 nm was obtained. **c,** Measured SHG conversion efficiency (dots) and the corresponding fitting function (solid line) obtained as the crystal temperature varied while the pump laser wavelength was fixed at 1079.27 nm. The center crystal temperature of 30.54°C with an FWHM of 11.2°C was obtained.

beams. Here, the polarization directions $y$ and $z$ represent horizontal and vertical, respectively. We measured the horizontally polarized SH beam generated by pumping a 20-mm-long KTP crystal with a diagonally polarized laser. Supplementary Figure 5**a** shows the obtained SHG conversion efficiency by measuring the power of the SH beam as we vary the temperature of the KTP crystal and the wavelength of the laser. The blue line represents the case where we maintain a temperature of 30°C while varying the wavelength. The measured data and its fitting function for this case are shown in Supplementary Fig. 5**b**. We used the sinc-squared function to obtain the fitting curve, as the generation rate of the SH beam follows Supplementary Eq. (2). The FWHM of the fitting function $\Delta\lambda$ is 0.32 nm. This result is consistent with the expected spectral bandwidth of the down-converted photons as shown in Supplementary Fig. 2**a**. The difference between their center wavelengths is 0.36 nm. Supplementary Figure 5**c** shows our experimental results when the laser operates at 1079.27 nm and the temperature is varied. This is indicated by the red line in Supplementary Fig. 5**a**. The FWHM of 11.2°C indicates the robustness of the SPDC process in a bulk KTP crystal against thermal instability in the external environment.

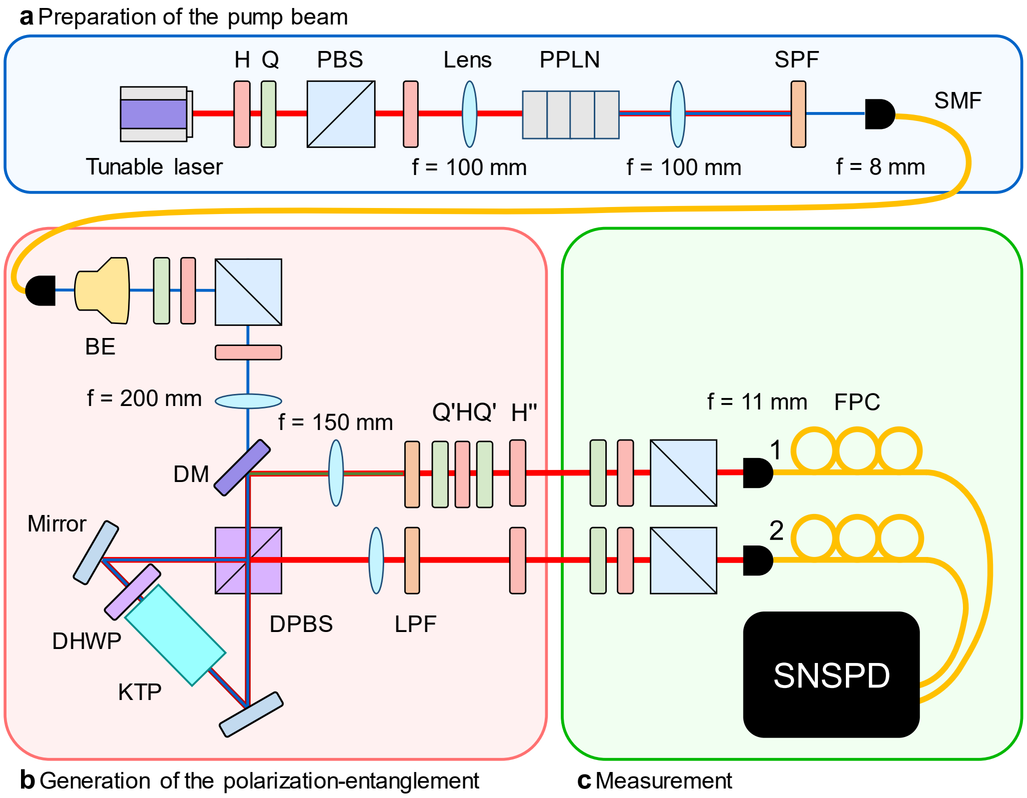


Supplementary Figure 6. **Experimental setup for generating polarization-entangled photon pairs via the SPDC process with Type-II NCPM in a bulk KTP crystal. a,** We prepare the pump beam using type-0 SHG process in a PPLN crystal. The SH beam at 539.64 nm is obtained by pumping a 40-mm-long PPLN crystal with a frequency-tunable external diode cavity laser at 1079.27 nm. **b,** The polarization-entangled photon pairs are generated at the polarization Sagnac interferometer (PSI) configuration with a 20-mm-long bulk KTP crystal [7]. We can prepare Bell states $|\phi^{\pm}\rangle = (|HH\rangle \pm |VV\rangle)/\sqrt{2}$ and $|\psi^{\pm}\rangle = (|HV\rangle \pm |VH\rangle)/\sqrt{2}$ by adjusting the angles of H$''$ and H in a set of Q$'$HQ$'$. **c,** We measured the generated photon pairs using the SNSPD. A set of H, Q, and PBS is located to perform projection measurement of the quantum state tomography (QST). H: half-waveplate; Q: quater-waveplate; PBS: polarization beam splitter; PPLN: periodically-poled lithium niobate; SPF: short pass filter; BE: beam expander; DM: dichroic mirror, DWHP: dual wavelength half-waveplate for 540 nm and 1080 nm, DPBS: dual wavelength polarization beam splitter for 540 nm and 1080 nm, KTP: potassium titanyl phosphate, LPF: long pass filter, Q$'$: quater-waveplate oriented at 45° FPC: fiber polarization controller, SNSPD: superconducting nanowire single photon detector.

### B. Experimental setup

Supplementary Figure 6 depicts the schematic diagram of our experimental setup to generate the polarization-entangled photon pairs via Type-II NCPM in a KTP crystal. As shown in Supplementary Fig. 6**a**, the frequency-tunable external cavity diode laser operating at 1079.27 nm is used to pump a 40-mm-long type-0 periodically-poled lithium niobate (PPLN) crystal to obtain its SH beam. The poling period of the PPLN crystal is 6.9 μm. The theoretical prediction for the RMS width of the obtained SH beam is 0.022 nm. After the laser beam is blocked by a short-pass filter (SPF), we coupled the SH beam into a single-mode fiber (SMF) to filter its spatial mode.

Polarization-entangled photon pairs are generated in the polarization Sagnac interferometer (PSI) using a 20-mm-long bulk KTP crystal [7] as shown in Supplementary Fig. 6**b**. The PSI consists of a dual wavelength polarization beam splitter (DPBS), a dual wavelength half-wave plate (DHWP) with an optic axis of 45°, and two mirrors. The KTP crystal is located at the center of the interferometer. The pump beam is focused to a spot with a beam waist $w_0 = 40$ μm at the center of the KTP crystal using a beam expander (BE) and a lens with a focal length of 200 mm. After orienting its polarization state as $|D\rangle$, the pump beam propagates into the PSI. The pump beam is divided into horizontal ($|H\rangle$) and vertical ($|V\rangle$) components at the DPBS, which traverse the PSI in clockwise and counterclockwise directions, respectively. The polarization state of the $|V\rangle$ components of the pump beam is rotated to horizontal by a DHWP. Then, the KTP crystal in the PSI is bidirectionally pumped to generate orthogonally polarized signal and idler photon pairs via the Type-II SPDC process. The generated counterpropagating photon pairs are combined at the DPBS. The signal (idler) photon and its counterpropagating signal (idler) photon propagate in the output modes of the PSI, denoted as 1 and 2 in Supplementary Fig. 6**c**. The produced polarization-entangled two-photon state is expressed as:

$$|\Psi\rangle = \frac{1}{\sqrt{2}}(|H_1V_2\rangle + e^{i\varphi}|V_1H_2\rangle), \tag{12}$$

where $\varphi$ represents the relative phase between two states, which can be fully adjustable by a set of Q′HQ′, consisting of two 45°-rotated quater-wave plates (QWP) and HWP. Q′HQ′ is located in mode 1. H′′ located in both modes rotate the polarization state of the photons to prepare four maximally entangled Bell states: $|\phi^{\pm}\rangle = (|HH\rangle \pm |VV\rangle)/\sqrt{2}$ and $|\psi^{\pm}\rangle = (|HV\rangle \pm |VH\rangle)/\sqrt{2}$.

The generated photon pairs are projected into different polarization bases and measured by the superconducting nanowire single photon detectors (SNSPDs) as shown in Supplementary Fig. 6**c**. A set of QWP, HWP, and PBS is located to perform quantum states tomography (QST) for full characterization of the generated state. An aspheric lens with $f = 11$ mm was used to couple the projected photon pairs into an SMF connected with an SNSPD. We optimized the detection efficiency of each SNSPD channel as ∼40% using a fiber polarization controller (FPC).

### C. Hong-Ou-Mandel experiment

We performed the Hong-Ou-Mandel (HOM) experiment to verify the indistinguishability of the generated photon pairs. We obtained the HOM interference fringes for photon pairs generated from $|H\rangle$ and $|V\rangle$ components of the pump beam divided at the DPBS, respectively. The measured coincidence counts for each input states are shown in Supplementary Fig. 7. We obtained HOM visibilities of 0.990±0.004 and 0.999±0.002 for the $|H\rangle$ and $|V\rangle$ input states, respectively.

### D. Quantum state tomography

Supplementary Figure 8 shows the real and imaginary parts of the reconstructed density matrices for the prepared four polarization-entangled Bell states. To quantify and estimate the properties of the produced two-photon entangled states, we calculated the three parameters from the reconstructed density matrices: purity ($\mathcal{P}$), concurrence ($\mathcal{C}$), and fidelity ($\mathcal{F}$) [8]. The obtained parameters are summarized in Table I in the main text. Since we obtained the parameters of $\mathcal{P} \geq 0.9887$, $\mathcal{C} \geq 0.9869$, and $\mathcal{F} \geq 0.986$, we can confirm that the prepared polarization-entangled photon states are very close to the ideal Bell states.

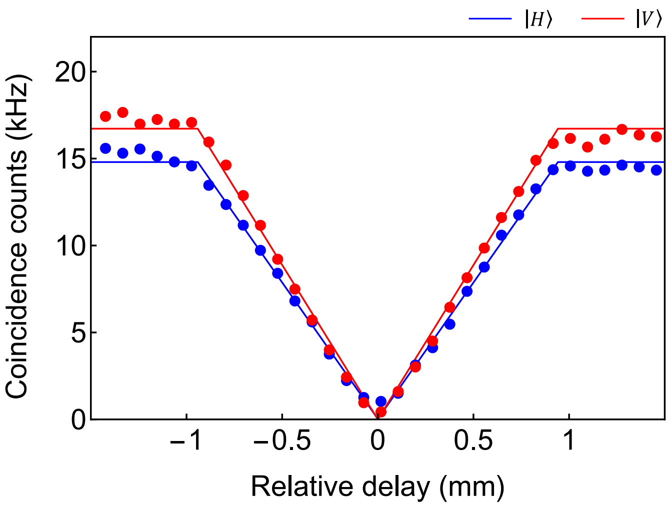


Supplementary Figure 7. **HOM interference.** We observed the HOM interferences for the photon pairs generated from a KTP crystal pumped by the $|H\rangle$ and $|V\rangle$ components of the pump beam. These components are separated at the DPBS as shown in Supplementary Fig. 6**b**. The fitting curve is obtained from the measured coincidence counts (dots). We assumed Poisson statistics to estimate the error bars corresponding to one standard deviation, which are represented in the graph but are too small to be visible. The obtained HOM visibilities are 0.990±0.004 and 0.999±0.002 for the $|H\rangle$ and $|V\rangle$ components of the pump beam, respectively. The errors correspond to one standard deviations.

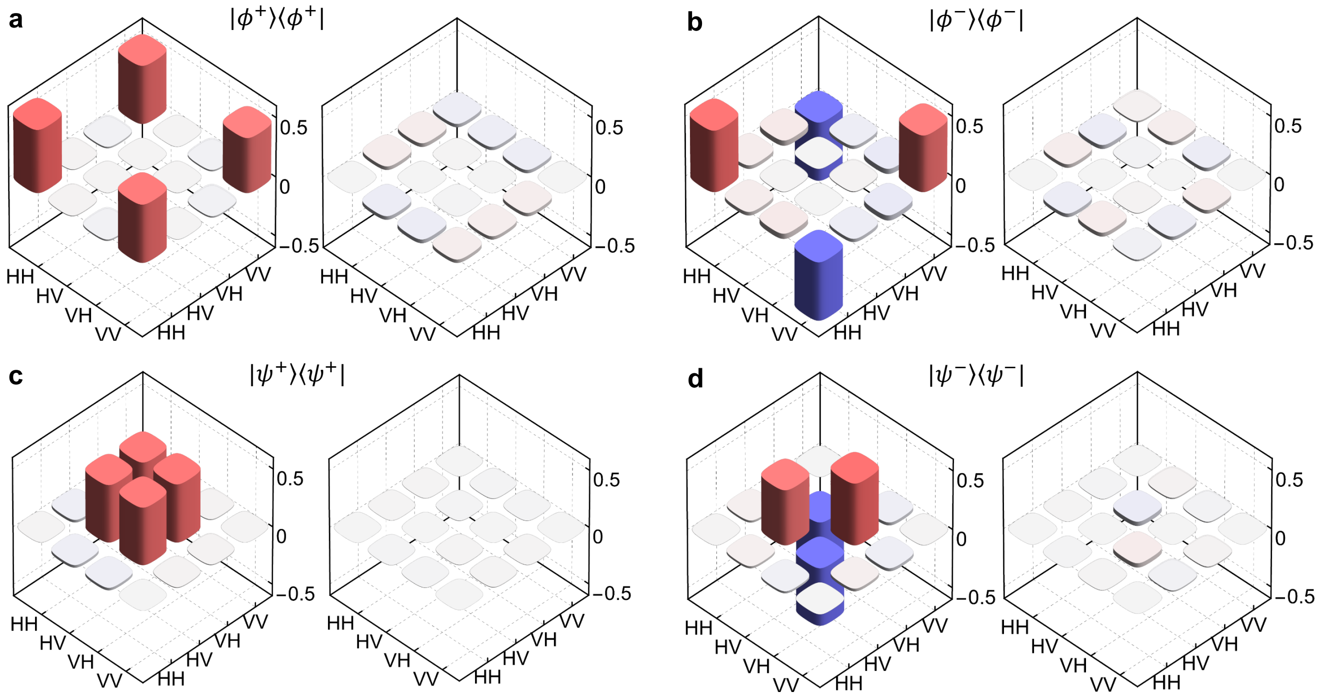


Supplementary Figure 8. **Reconstructed density matrices of the four Bell states.** The real (left) and imaginary (right) parts of the reconstructed density matrices for the prepared states. **a,** $|\phi^+\rangle$, **b,** $|\phi^-\rangle$, **c,** $|\psi^+\rangle$, and **d,** $|\psi^-\rangle$.


[1] Emanueli, S. & Arie, A. Temperature-dependent dispersion equations for $KTiOPO_4$ and $KTiOAsO_4$. *Appl. Opt.* **42**, 6661–6665 (2003).

[2] Kato K. and Takaoka, E. Sellmeier and thermo-optic dispersion formulas for KTP. *Appl. Opt.* **41**, 5040–5044 (2002).

[3] Zhu, J. et al. Demonstration of measuring sea fog with an snspd-based lidar system. *Sci. Reports* **7**, 1–7 (2017).

[4] Xue, L. et al. Satellite laser ranging using superconducting nanowire single-photon detectors at 1064 nm wavelength. *Opt. Lett.* **41**, 3848–3851 (2016).

[5] Wang, Z., Malaney, R. & Burnett, B. Satellite-to-earth quantum key distribution via orbital angular momentum. *Phys. Rev. Appl.* **14**, 064031 (2020).

[6] Kim, I., Lee, D. & Lee, K. J. Numerical investigation of high-purity polarization-entangled photon-pair generation in non-poled KTP isomorphs. *Applied Sciences* **11**, 565 (2021).

[7] Kim, T., Fiorentino, M. & Wong, F. N. C. Phase-stable source of polarization-entangled photons using a polarization Sagnac interferometer. *Phys. Rev. A* **73**, 012316 (2006).

[8] James, D. F., Kwiat, P. G., Munro, W. J. & White, A. G. Measurement of qubits. *Phys. Rev. A* **64**, 052312 (2001).
